# Supplementary material for: Trust-region approximation of extreme trajectories in power system dynamics
Source: arXiv:2106.16132 source file (2022-02-08)
Supplement: Supplementary file 1 [file appendixA.tex]

This appendix contains a matrix formulation of the first- and 
second-order sensitivity equations, a description of the implementation of a backward Euler scheme for their integration, and an experimental validation with finite differences.
